# Supplementary material for: Streaking temporal double slit interference by an orthogonal two-color laser field
Source: arXiv:1503.02658 source file (2015-03-09)
Supplement: Supplementary file 1 [file supplemental.pdf]

# Streaking temporal double slit interference by an orthogonal two-color laser field: supplemental material

Martin Richter,[1] Maksim Kunitski,[1] Markus Schöffler,[1] Till Jahnke,[1]
Lothar P.H. Schmidt,[1] Min Li,[2] Yunquan Liu,[2, 3] and Reinhard Dörner[1]

[1] *Institut für Kernphysik, Goethe-Universität Frankfurt, 60438 Frankfurt am Main, Germany*
[2] *State Key Laboratory for Mesoscopic Physics and Department of Physics, Peking University, Beijing 100871, People's Republic of China*
[3] *Collaborative Innovation Center of Quantum Matter, Beijing 100871, China*

In the supplemental material a more detailed description of the experimental setup is given and the method for the determination of the absolute phase between the two colors is shown.

## EXPERIMENTAL SETUP

In our experiment the perpendicularly polarized second harmonic field (390 nm) was generated in a 200 $\mu$m $\beta$-Barium borate-crystal ($\beta$-BBO) by frequency doubling of a 780 nm laser pulse (KMLabs Dragon, 40 fs FWHM) at a rate of 8 kHz in a collinear configuration. The temporal overlap between the two pulses was achieved by compensating for the different group velocities of the two colors with a 6 mm $\alpha$-BBO crystal (X-cut) and a pair of fused silica wedges. Because of this large amount of dispersive material in the beam path the temporal length of the 780 nm and 390 nm pulses was stretched to 55 fs and 70 fs, respectively. The phase between the two colors has been tuned by varying the amount of glass in the two-color beam path. Because of the phase drift due to air humidity and temperature fluctuations a continuous phase scan was performed to be able to correct for this drift in the offline analysis. The absolute phase between the two colors was retrieved by considering the streaking of the low energy electrons (born at the maximum of the 780 nm electric field) along the polarization direction of the 390 nm laser field. The total OTC field is given by

$$\vec{E} = E_{z,780}\cos(\omega t)\vec{e}_z + E_{y,390}\cos(2\omega t + \phi)\vec{e}_y. \tag{1}$$

The intensity of the 780 nm field ($1.4 \cdot 10^{14}\mathrm{W/cm^2}$) was estimated according to the $2U_P$ energy cutoff in the electron energy spectrum ($p_z^{cutoff} = 2\sqrt{U_P} = 1.08\mathrm{au}$). The intensity of the 390 nm pulse ($1.3 \cdot 10^{13}\mathrm{W/cm^2}$) is estimated by a comparison to the QTMC-simulation.

The OTC pulses are focused into a supersonic gas jet of argon atoms and the three-dimensional (3D) momentum spectra of the resulting singly charged ions and electrons are measured in a COLTRIMS setup [1]. An electric field of 10.8 V/cm and a collinear magnetic field of 8 Gauss guided the electrons onto a time and position sensitive micro-channel plate detector [2]. For electrons with momenta up to 1.5 au this configuration allows to detect all electrons emitted within a solid angle of $4\pi$. The polarization of the 780 nm field was chosen to lie along the time-of-flight axis.

## ABSOLUTE PHASE

Experimentally, we insert a wedge and record its position x. The absolute phase difference $\Delta\phi = \phi_{780nm} - \phi_{390nm}$ between the two colors is linear to the wedge position, $\Delta\phi = ax + b$, and we need to determine the constants a and b. In our experiment we have continuously scanned the wedge positon x and recorded its value for each event. This allows us to create the plot in Fig. 1 from which we obtain the constants a and b. The horizontal axis shows the wedge position, the vertical axis the momentum component of the emitted electron along the direction of the 390 nm field (i.e. the y-direction). We have selected only those events for which the momentum component along the 780 nm field is zero ($abs(p_z) < 0.05au$). This selects electrons mainly born close to (and symmetric to) the maximum of the 780 nm field ($\phi_{780nm} = 0$). As shown in the figure there are two main features in the distribution of $p_y$. Firstly, there is a narrow line at $p_y = 0$ which is independent of the wedge position. These are Coulomb focused electrons which are not in the focus of the present paper. The second prominent feature is a clear sinusoidally oscillating contribution. These are the electrons which are streaked by the 390 nm field, this oscillating feature directly shows the vector potential of the 390 nm field (relative to the fixed phase $\phi_{780nm} = 0$). From the period of this feature we gather the constant a. The phase offset b is determined from the maxima and zero crossings of the streaked component as indicated by the vertical lines.

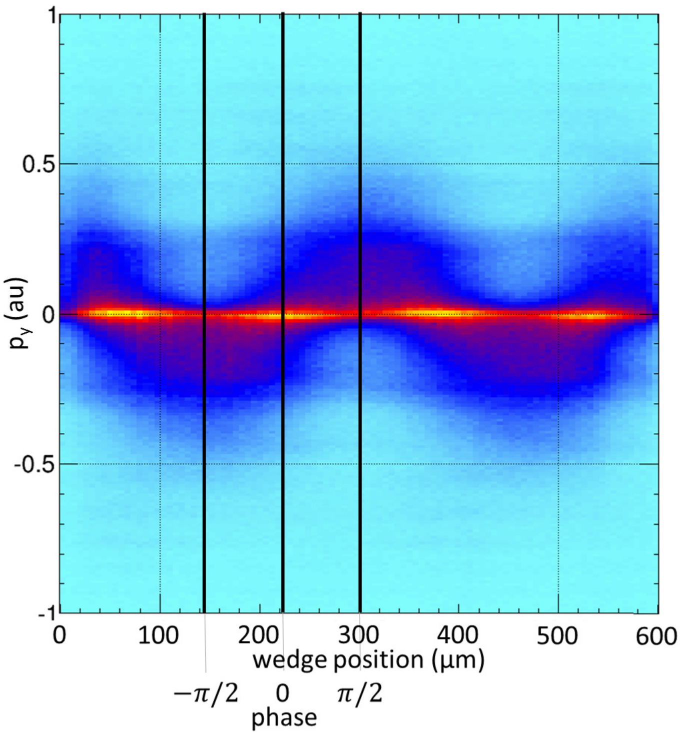


FIG. 1. The wedge position x versus the momentum component $p_y$ of the emitted electrons along the direction of the 390 nm field is plotted. Only events within a small momentum range along the 780 nm field direction are taken into account $(abs(p_z) < 0.05au)$. The black vertical lines represent the phases extracted from the plot.


[1] R. Dörner, V. Mergel, O. Jagutzki, L. Spielberger, J. Ullrich, R. Moshammer, and H. Schmidt-Böcking", Physics Reports **330**, 95 (2000).

[2] O. Jagutzki, A. Cerezo, A. Czasch, R. Dörner, M. Hattas, M. Huang, V. Mergel, U. Spillmann, K. Ullmann-Pfleger, T. Weber, H. Schmidt-Bocking, and G. Smith, Nuclear Science, IEEE Transactions on **49**, 2477 (2002).
